# Supplementary material for: Facilitating a 3D granular flow with an obstruction
Source: arXiv:2411.11264 source file (2024-11-18)

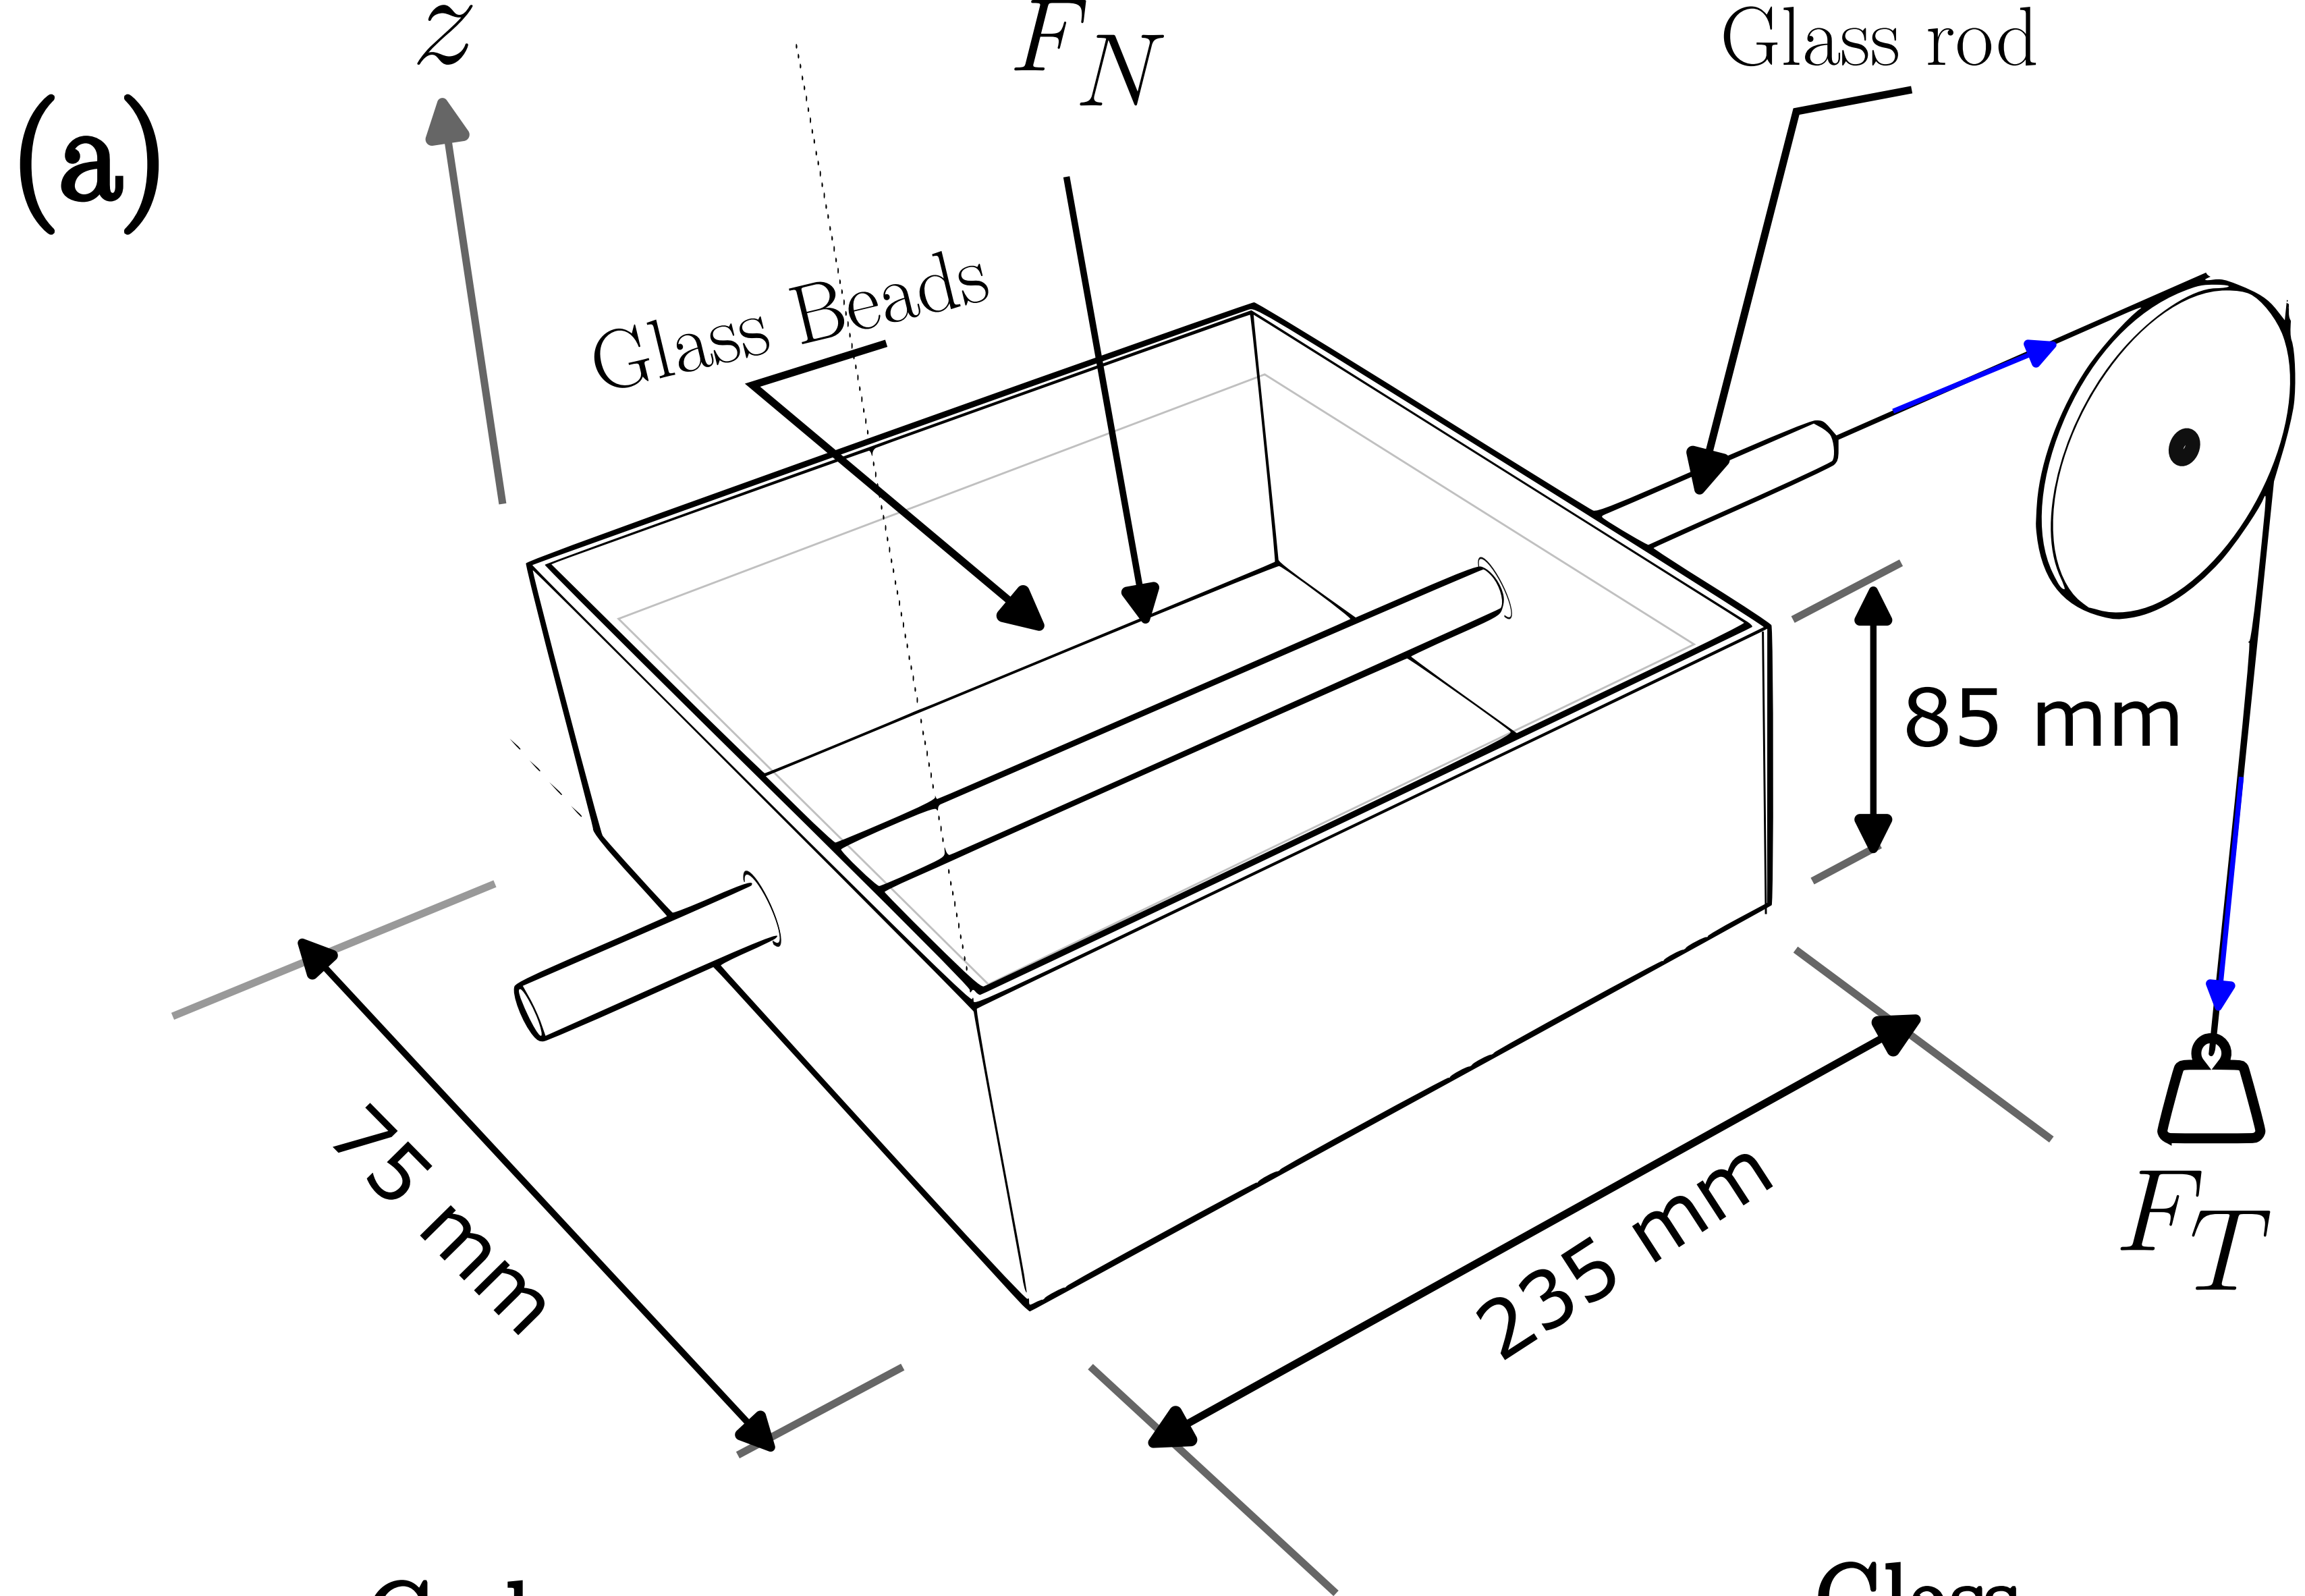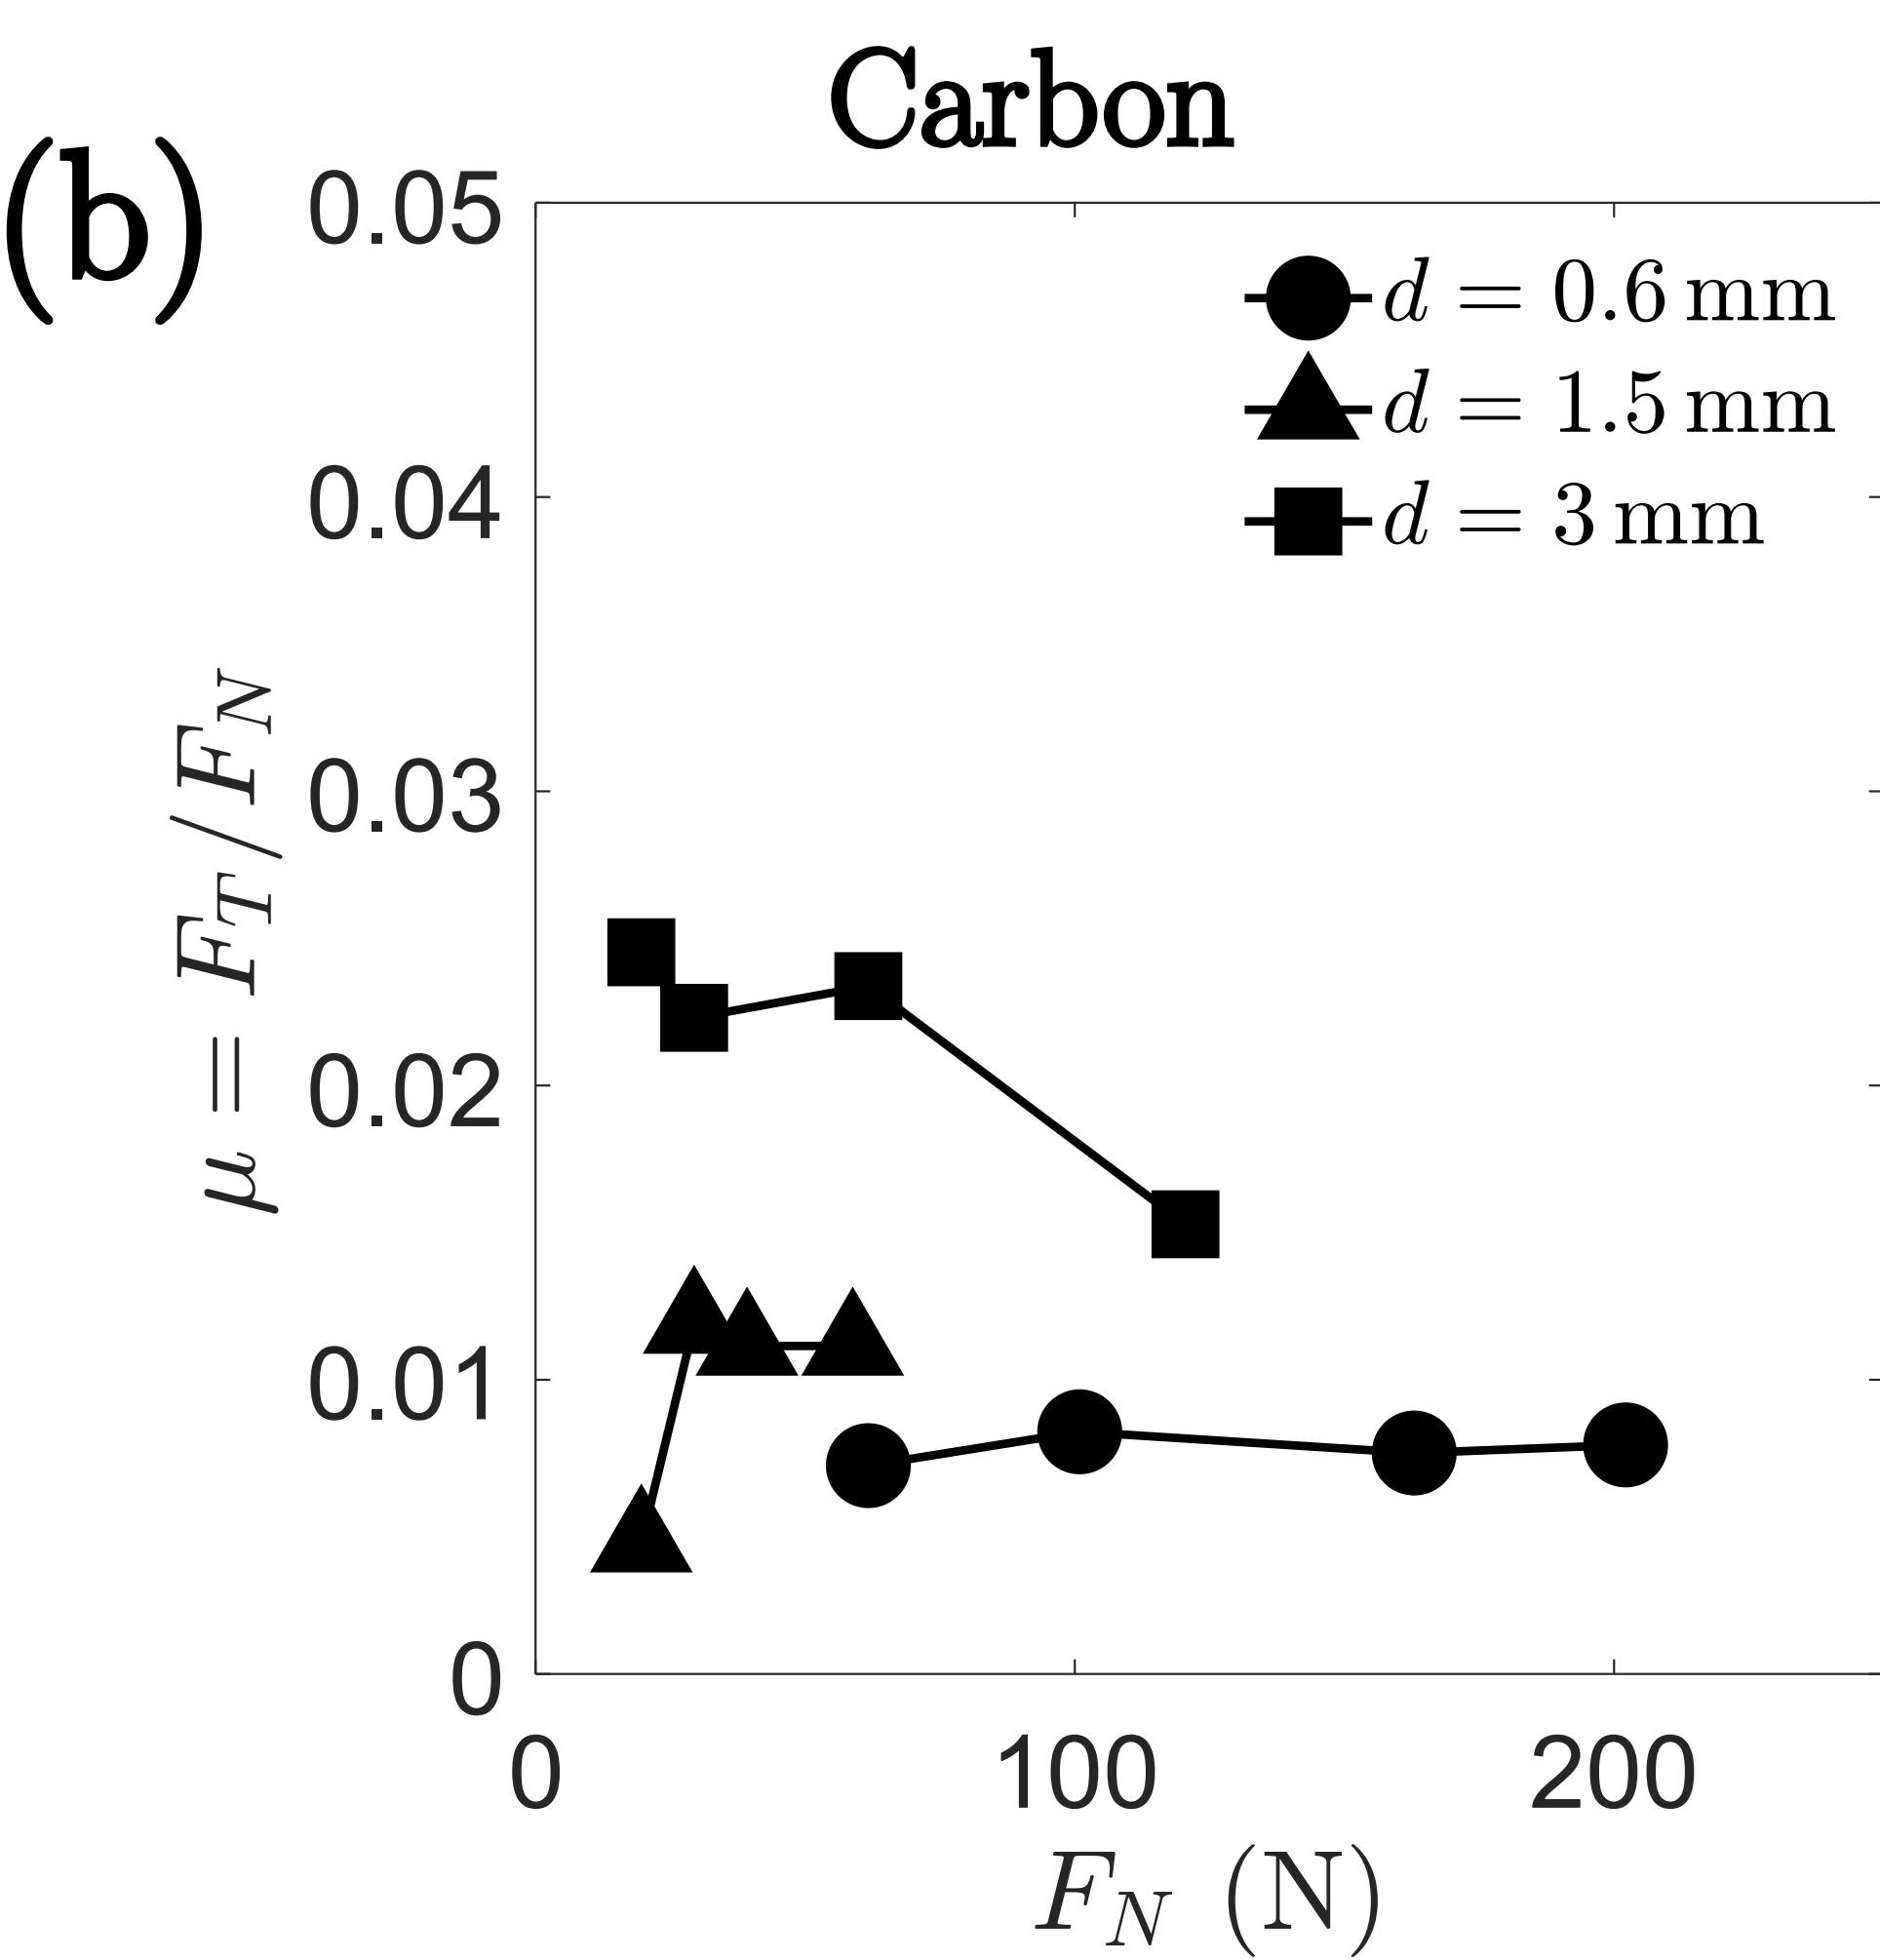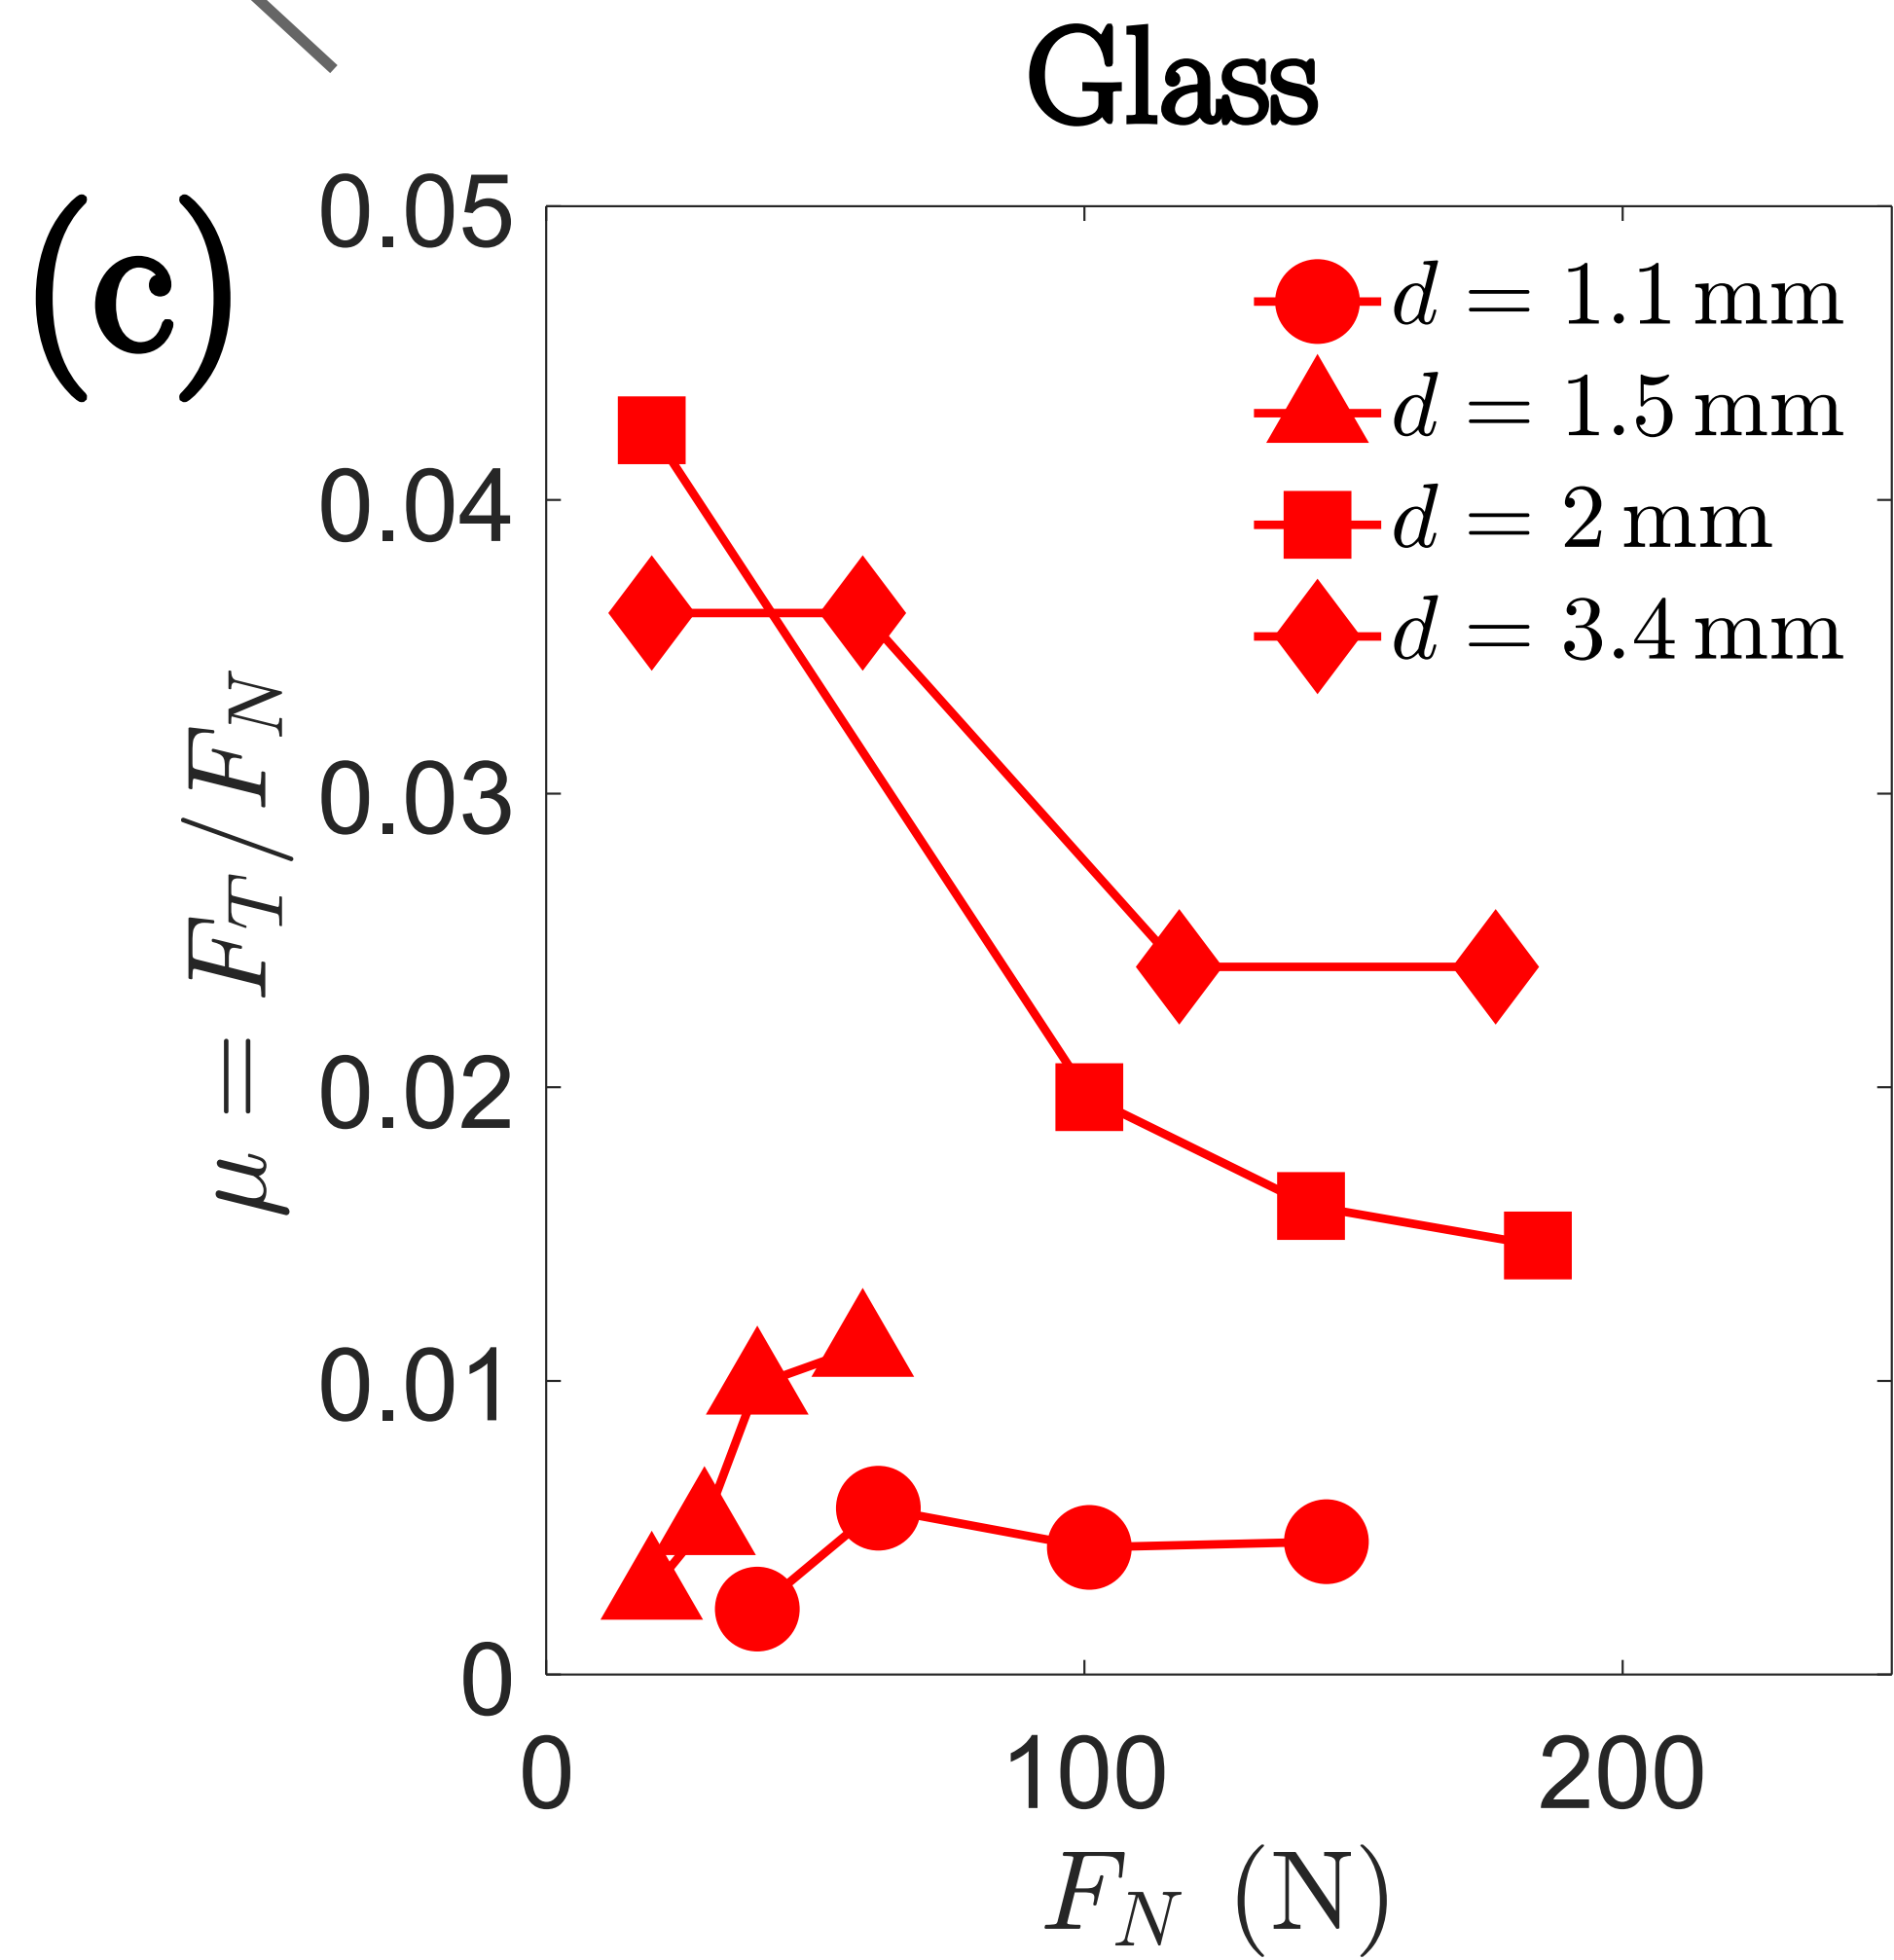

Supplement: Supplementary file 2 [file suppl_fric_measurement_new.pdf]
